# Supplementary material for: Spatially Modulated Superfluid State in Two-Dimensional $^4$He Films
Source: arXiv:2108.06623 source file (2021-08-14)
Supplement: Supplementary file 1 [file 2021Choi_4He_Films_SM_revised_2nd.pdf]

# Supplemental Material for "Spatially Modulated Superfluid State in Two-dimensional $^4$He"

J. Choi,[1] A. A. Zadorozhko,[1] J. Choi,[1] and E. Kim[1]

[1] *Department of Physics, Korea Advanced Institute of Science and Technology (KAIST), 291 Daehak-ro, Yuseong-gu, Daejeon 34141, Republic of Korea*

## I. EXPERIMENTAL DETAILS

**Dosing of $^4$He atoms**: To grow $^4$He films on a graphite substrate, ultrahigh-purity $^4$He gas with a $^3$He impurity concentration of 0.6 ppb contained in a high-pressure cylinder was systematically dosed. A gas handling system with a fixed-volume space was constructed for the accurate dosing of $^4$He gas. All capillaries, valves, and fittings in the gas handling system were made for a high-pressure usage. First, we transfer the $^4$He gas from the high-pressure gas cylinder to the fixed volume through both a liquid nitrogen and a helium trap. Pressure inside the gas handling system was monitored by a Baratron pressure transducer. Then, the $^4$He gas was admitted to the sample cell inside a cryostat by opening a HIP valve on the top flange. When the pressure reads from the Baraton transducer reached to the desired value, the adimission of $^4$He was stopped by closing the HIP valve. The number of $^4$He atoms transferred to the sample cell in each dosing was calculated from the pressure change of the $^4$He gas remained in the gas handling system and the ideal gas law. To accurately calculate the number of $^4$He atoms introduced, temperature of the $^4$He gas inside the sample cell and the high-pressure side outside of the fridge were measured with high precision. In order to prevent any development of pressure gradient and to secure a clearance, we installed the filling line straight through from the 4-K flange to the mixing chamber of our dilution refrigerator.

**Annealing $^4$He films**: After the admission of new $^4$He atoms to the sample cell, $^4$He films were annealed at high temperature for uniformly distributing the introduced $^4$He atoms over the substrate surface. Due to different absorption potential for each layers, different annealing conditions were used as shown in Supplementary Table 1. After warming up the fridge to the desired annealing temperature slowly, we waited at least $\sim$3 hours before cooling down. Then, we cooled down the fridge and the sample cell for at least 10 hours. A resistor heater wound around the filling capillary was turned on while dosing to prevent any unwanted $^4$He films growth.

***in-situ* pressure gauge**: A diaphragm-type pressure gauge was mounted on the experimental stage for accurate calibration of vapor pressure inside the sample cell. Its design is similar to that used in the previous TO experiment [1]. An aluminized Kapton sheet with 25-$\mu$m thickness was employed as a diaphragm in between two electrodes. We also put another 7-$\mu$m ring-shaped Kapton layer as a spacer. The capacitance between the two electrodes measured by AH2550 capacitance bridge is typically around 55 pF. The pressure gauge was calibrated at high temperature in a range of 0 $\sim$ 0.2 Torr where it shows a linear response to increased $^4$He vapor pressure. Its sensitivity $\delta P$ was calculated to $2.5 \times 10^{-7}$ Torr, comparable to the pressure gauge used in Ref. [2].

**Supplementary Table** 1. Summary of annealing conditions for each $^4$He layers.

| Layer | Coverage | Annealing temperature | Waiting time | Cooling rate |
|---|---|---|---|---|
| first layer | $0 < n < 11.1$ atoms/nm$^2$ | 10 K | 3 hours | 1 K/hr |
| second layer | 11.1 atoms/nm$^2$ $< n <$ 20.4 atoms/nm$^2$ | 4 K | 3 hours | 0.4 K/hr |
| third layer | $n > 20.4$ | 2 K | 3 hours | 0.2 K/hr |

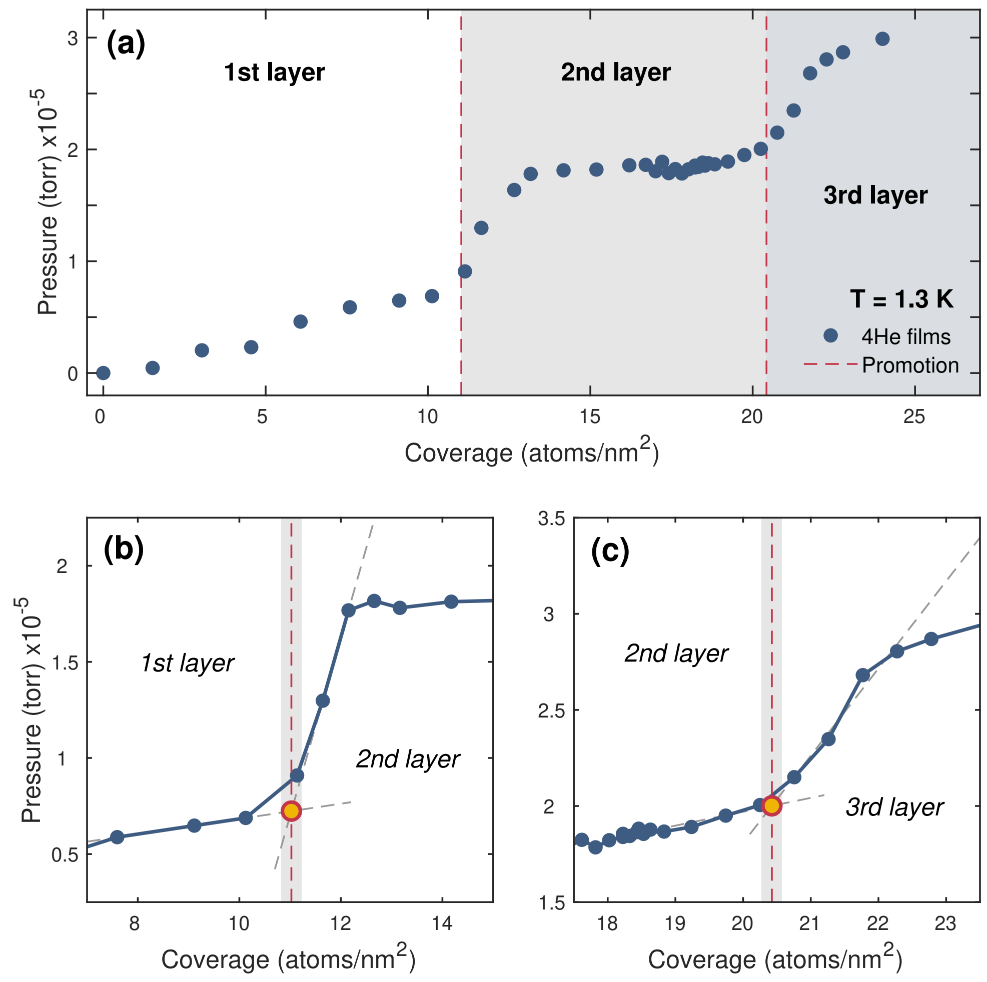


**Supplementary Fig.** 1. **Layering transitions in two-dimensional $^4$He films on graphite** (a) Vapor pressure isotherm of $^4$He films adsorbed on Grafoil at 1.3 K. The red dashed lines indicate layer promotion coverages to the second and third layer. Determination of the layer promotion coverage to (b) the second layer and (c) the third layer. The red circles represents the layer-promotion coverage determined by linear extrapolation (grey dashed lines) of the vapor pressures measured before and after the layering transition. The shaded regions correspond to the uncertainty of each layer-promotion coverage.

**Grafoil substrate characterization**: We employed 11 Grafoil disks as a substrate. To convert the number of admitted $^4$He atoms into the absolute coverage $n$, we need to accurately determine the total surface area of the Grafoil substrate. In principle, the surface area of substrate can be inferred by a sudden jump in $^4$He vapor pressure at low temperature, due to the structural transition to the $\sqrt{3} \times \sqrt{3}$ commensurate solid phase, expected at 6.37 atoms/nm$^2$. However, this signature is hardly detectable at relevant temperature range of this measurement. Thus, $N_2$ or Kr gas has been widely used to identify the $\sqrt{3} \times \sqrt{3}$ solid phase. Fig. 1(b) shows the vapor pressure isotherm of $N_2$ obtained at a fixed temperature of 78 K. The nearly constant vapor pressure between 82 to 84 $\mu$mol upon adding $N_2$ atoms is a signature of the formation of $\sqrt{3} \times \sqrt{3}$ solid phase. When its formation is completed at 6.37 atoms/nm$^2$, the slope of $N_2$ vapor pressure shows a discontinuous change. Even though its signature is somewhat rounded probably due to the nonuniform effective size distribution of individual crystallite arrays of the Grafoil substrate, the completion of $\sqrt{3} \times \sqrt{3}$ solid phase is clearly visible in Fig. 1(b). To determine the exact completion point, we extrapolate the two different slopes before and after the completion of $\sqrt{3} \times \sqrt{3}$ solid phase and find a point where two slopes meet (red dashed line). From this method, we obtained $7.99 \pm 0.06$ m$^2$ for the Grafoil substrate used in our experiment. The uncertainty is determined by the shaded region in Fig. 1(b). The surface area of filling capillary inside the fridge was corrected.

**Layer-by-layer growth of $^4$He**: Grafoil, an exfoliated graphite, inevitably contains various structural defects such as cracks, steps, and dead-ends. Thus, it forms a random network of poorly connected crystallite arrays with a limited surface coherence of 10∼20 nm [3]. This poor connectivity and nonuniform surface on a macroscopic length scale could hinder development of a long-range correlation and degrade sensitivity of torsional oscillator responses to superfluid mass decoupling [1]. Thus, it is important to assess the quality of Grafoil substrate used in our experiment. Observation of layer-by-layer growth of $^4$He is a good indicator of a clean substrate surface. Supplementary Fig. 1 shows successive layering transitions observed in $^4$He films grown inside our torsional oscillator. The vapor pressure of $^4$He films were measured by the *in-situ* pressure gauge installed on the filling capillary connected to the sample cell containing Grafoil disks. As shown in Supplementary Fig. 1(a), we observed two clear discontinuous jumps in the $^4$ vapor pressure indicating the layering transition of $^4$He films. To extract the layer-promotion coverage more accurately, we extrapolate the several data points before and after the layer promotion to the second and third layer, as shown in Supplementary Figs. 1(b) and 1(c), respectively. As a result, the layer-promotion coverage was calculated to be $11.1 \pm 0.2$ and $20.4 \pm 0.2$ atoms/nm$^2$ for the promotion to the second and third layer, respectively.

## II. RIGID DOUBLE-FREQUENCY TORSIONAL OSCILLATOR

Two-fluid model stated the total mass density $\rho$ of superfluid system consists of "normal density", $\rho_\mathrm{n}$, and "superfluid density", $\rho_\mathrm{s}$ [4, 5] below the critical temperature $T_\mathrm{c}$. Andronikashvili-type torsional oscillator (TO) technique is one of the most direct experimental probe of the superfluid density $\rho_s$ [6]. Its resonant period $P$ is determined by $\sqrt{(I_\mathrm{TO}+I_\mathrm{He})/K}$, where $I_\mathrm{TO}$ and $I_\mathrm{He}$ are the rotational inertia of a TO body and $^4$He films, and $K$ is the elastic modulus of a torsion rod. Due to its viscousless nature, the superfluid component decouples from the oscillation of the TO body below $T_\mathrm{c}$ and hence does not contribute on $I_\mathrm{He}$. This "missing" inertia $\delta I_s$ leads to a decrease in the resonant period of TO, $\delta P$. The superfluid density $\rho_\mathrm{s}(T,n)$ is then determined by $\delta P(T,n)/\Delta P(n)$, where $\Delta P(n)$ is the period increase at 500 mK, due to the mass of $^4$He atoms added to a substrate at a given coverage $n$.

However, TO studies on possible supersolid phase in bulk solid $^4$He [7–9] reveal that TOs are not only sensitive to "missing inertia" $\delta I_s$ due to the superfluid transition, but also the change in the elastic modulus $K$ of the TO body due to viscoelastic effects [10–14]. Since the elastic modulus of TO components and solid $^4$He contribute to the combined elastic stiffness $K$, the stiffening in the elastic modulus of solid $^4$He observed at low temperature $\delta K_\mathrm{el}$ [15] leads to a reduction in a TO period. Furthermore, various nonlinear viscoelastic coupling mechanisms between the TO and solid $^4$He significantly enhance this contribution and produce superfluid-mimicking period reduction, $\delta P_\mathrm{el}$. It was known to be notoriously difficult to distinguish the contribution of genuine superfluid and viscoelastic effects on the TO period change $\delta P$. Two recipes have been suggested: (a) fabricating a specially designed TO that suppresses the viscoelastic contributions [13, 16, 17] (b) investigating frequency dependence of $\delta P$ [10, 14, 16, 17].

First, we constructed a TO that can be operated at two different frequencies to study the frequency dependence of the period reduction $\delta P$. As shown in Fig. 1(a), our TO has a double-pendulum structure. The upper torsional mass (sample cell) $I_1$ and the lower torsional mass (electrode plate) $I_2$ that connected through two torsional rods with an elastic modulus of $K_1$ and $K_2$, respectively, in series behave as a double-pendulum mass-spring system. Thus, the TO exhibits two eigenfrequencies:

$$f_\pm^2 = \frac{I_1(K_1+K_2)+I_2K_1}{8\pi^2 I_1 I_2}\left[1 \pm \sqrt{\frac{4I_1I_2K_1K_2}{\{I_1(K_1+K_2)+I_2K_1\}^2}}\right]. \tag{1}$$

Here, $f_-$ and $f_+$ are the lowest and the second lowest eigenfrequencies that correspond to two different torsional motions. In the lowest frequency (1st, low mode), both the sample cell and electrodes oscillate *in-phase* or move in the same direction, whereas two masses oscillate *out-of-phase* or move in the opposite direction in the second lowest frequency (2nd, high mode). Our TO has the lowest and the second lowest torsional resonance at 511 and 1246 Hz, respectively. Based on this design, we could measure the superfluid density $\rho_s(T,n) = \delta P(T,n)/\Delta P(n)$ at two

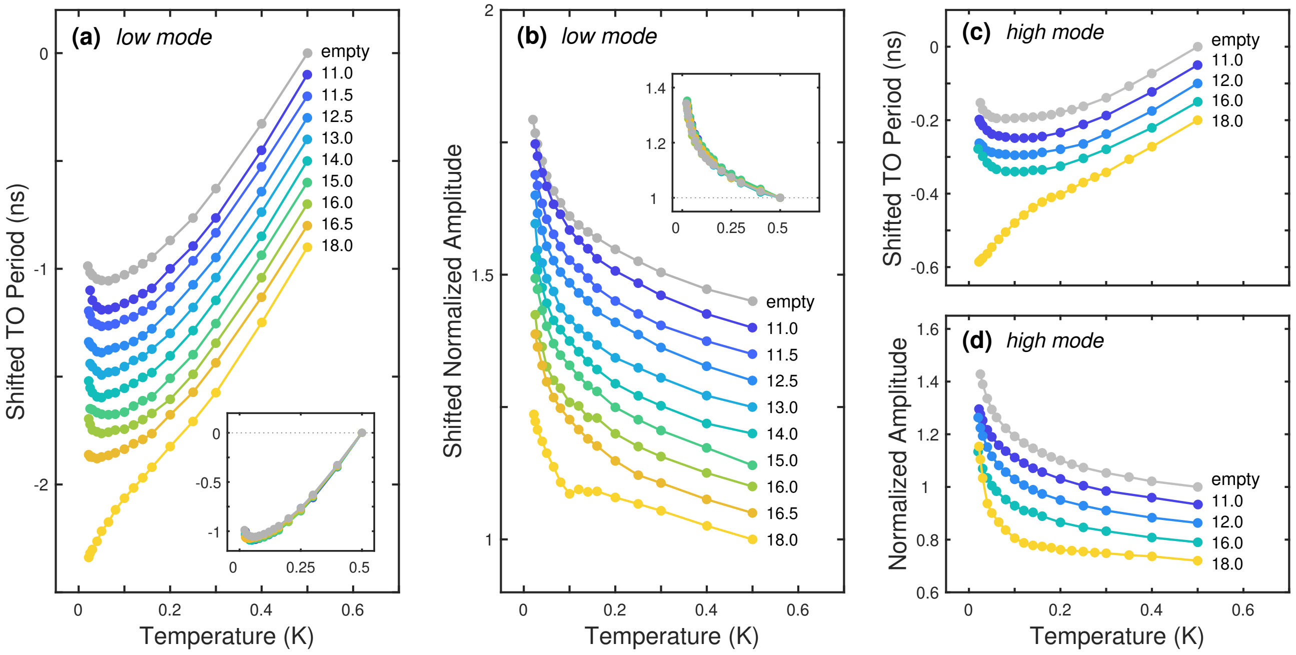


**Supplementary Fig.** 2. **Torsional oscillator (TO) responses for nonsuperfluid $^4$He films.** Temperature dependence of (a) period and (b) amplitude in the low-frequency mode of our rigid two-frequency TO containing nonsuperfluid (or inert) $^4$He films adsorbed on Grafoil. The TO periods measured at the coverages as indicated were vertically shifted for better comparison of high-temperature background. The TO amplitude curves are first normalized to their value measured at 500 mK and then vertically shifted. The insets of (a) and (b) show all temperature-dependent TO period and amplitude curves can be superimposed with each other, if vertically shifted. (c), (d) Same plots for the TO responses in the high-frequency mode, measured at different coverages as indicated.

different frequencies, $f_-$ and $f_+$. $\Delta P(n)$ is the period increase due to loading of $^4$He films measured at 500 mK. If the emergence of superfluidity is solely responsible for the TO response, the superfluid density measured at two different frequencies should be equivalent; $\rho_s(T \to 0) = \delta P_-/\Delta P_- = \delta P_+/\Delta P_+$. This relation was confirmed by our superfluid density measurement in the third layer where the existence of BKT superfluid has been established (see Supplementary Fig. 3). Other mechanisms such as viscoelastic property change [14, 15] or slippage of $^4$He atoms on substrate [18, 19], on the other hand, produce nontrivial frequency responses. For example, the viscoelastic stiffening of solid $^4$He induces a superfluid-mimicking period decrease $\delta P/\Delta P$ proportional to $f^2$, virtually indistinguishable from the genuine superfluid transition by single-mode TOs. Thus, the observation of frequency-independent $\rho_s$ is a distinctive evidence of genuine superfluid phase in the second layer of $^4$He films.

Second, we designed our TO by following a design principle satisfying the so-called “rigidity” criteria. An example of a rigid TO adopting the rigidity criteria was presented in our previous study on bulk solid $^4$He [16]. From our previous experience, rigid TOs show two typical characteristics: (a) High-temperature backgrounds are almost perfectly overlapped with that of empty-cell when vertically translated. Supplementary Fig. 2 shows temperature-dependent period and amplitude of our TO measured at different coverages $n$ before the superfluid critical coverage $n_c = 17$ atoms/nm$^2$. The typical temperature dependence of the TO without loading helium films reflects the elastic modulus change of the TO with varying temperature, which is called as an empty cell background [grey solid symbols in Supplementary Fig. 2(a)]. Upon the addition of non-superfluid helium films, the resonant period of the ideally rigid TO is raised without altering temperature dependence due to the rotational inertia increase in the torsion cell. Thus, high-temperature backgrounds obtained at different coverages are vertically translated by the mass loading of $^4$He atoms at a given coverage and can be superimposed with each other when vertically shifted, as shown in Supplementary Fig. 2(a). Accordingly, one can investigate the change in the TO response with superfluid $^4$He films in the torsion cell by subtracting the empty TO background. However, the temperature dependence of the period of

non-rigid TOs with non-superfluid film gets generally stiffer than those of the empty TO background and a "composite background" has been introduced to compensate a tilted linear background. This stiffening was attributed to the viscoelastic coupling of a non-rigid TO to $^4$He films and accompanied by non-monotonous change in the dissipation. Although the amount of $^4$He added to a TO was very small, a non-superfluid $^4$He films modified the temperature dependence of the TO response sharply [20]. As presented in Supplementary Fig. 2, all temperature-dependent period and amplitude curves in both frequency modes can be superimposed with each other, when vertically shifted. Below the critical coverage $n_c < 17$ atoms/nm$^2$, all curves measured with nonsuperfluid $^4$He films are almost identical to the empty-TO response (See insets). For the period and amplitude curves obtained in the presence of superfluid at 18.02 atoms/nm$^2$, high-temperature backgrounds are not altered by the viscoelastic contribution. The absence of "composite" background confirms that our TO is made to be rigid and provides an ideal environment of searching superfluidity in $^4$He films adsorbed on graphite.


[1] P. A. Crowell and J. D. Reppy, "Superfluidity and film structures in $^4$He adsorbed on graphite," Phys. Rev. B **53**, 2701–2718 (1996).

[2] G. Zimmerli, G. Mistura, and M. H. W. Chan, "Third-sound study of a layered superfluid helium," Phys. Rev. Lett. **68**, 60 (1992).

[3] R. J. Birgeneau, P. A. Heiney, and J. P. Pelz, "High resolution x-ray studies of monolayer krypton on varied forms of graphite," Physica B **109-110**, 1785–1795 (1982).

[4] L. Tisza, "Transport phenomena in helium II," Nature **141**, 913 (1938).

[5] W. Guo, M. La Mantia, D. P. Lathrop, and S. W. Van Sciver, "Visualization of two-fluid flows of superfluid helium-4," Proc. Natl. Acad. Sci. USA **111**, 4653–4658 (2014).

[6] E. L. Andronikashvili, "Direct observation of two kinds of motion in helium II," J. Phys. USSR **5**, 71–90 (1941).

[7] E. Kim and M. H. W. Chan, "Probable observation of a supersolid helilum phase," Nature **427**, 225 (2004).

[8] E. Kim and M. H. W. Chan, "Observation of superflod in solid helium," Science **305**, 1941 (2004).

[9] M. Boninsegni and N. V. Prokof'eV, "Supersolids: What and where are they?" Rev. Mod. Phys. **84**, 759 (2012).

[10] X. Mi and J. D. Reppy, "Anomalous behavior of of solid He in porous vycor glass," Phys. Rev. Lett. **108**, 225305 (2012).

[11] J. R. Beamish, A. D. Fefferman, A. Haziot, X. Rojas, and S. Balibar, "Elastic effects in torsional oscillators containing solid helium," Phys. Rev. B **85**, 180501(R) (2012).

[12] H. J. Maris, "Effect of elasticity on torsional oscillator experiments probing the possible supersolidity of helium," Phys. Rev. B **86**, 020502(R) (2012).

[13] D. Y. Kim and M. H. W. Chan, "Upper limit of supersolidity in solid helium," Phys. Rev. B **90**, 064503 (2014).

[14] J. D. Reppy, X. Mi, A. Justin, and E. J. Mueller, "Interpreting torsional oscillator measurements: effect of shear modulus and supersolidity," J. Low Temp. Phys. **168**, 175–193 (2012).

[15] J. Day and J. Beamish, "Low temperature shear modulus changes in solid $^4$He and connection to supersolidity," Nature **450**, 853–856 (2007).

[16] J. Choi, J. Shin, and E. Kim, "Frequency-dependent study of solid $^4$He contained in a rigid double-torus torsional oscillator," Phys. Rev. B **92**, 144505 (2015).

[17] J. Choi, T. Tsuiki, D. Takahashi, H. Choi, K. Kono, K. Shirahama, and E. Kim, "Reinvestigation of the rotation effect in solid $^4$He with a rigid torsional oscillator," Phys. Rev. B **98**, 014509 (2018).

[18] M. Hieda, T. Nishino, M. Suzuki, N. Wada, and K. Torii, "Slippage of nonsuperfluid helium films," Phys. Rev. Lett. **85**, 5142–5145 (2000).

[19] N. Hosomi and M. Suzuki, "Sliding friction of multilayer $^4$He films adsorbed on graphite," Phys. Rev. B **77**, 024501 (2008).

[20] G. Agnolet, D. F. McQueeney, and J. D. Reppy, "Kosterlitz-Thouless transition in helium films," Phys. Rev. B **39**, 8934 (1989).

[21] D. J. Bishop and J. D. Reppy, "Study of the superfluid transition in two-dimensional $^4$He films," Phys. Rev. B **22**, 5171–5185 (1980).

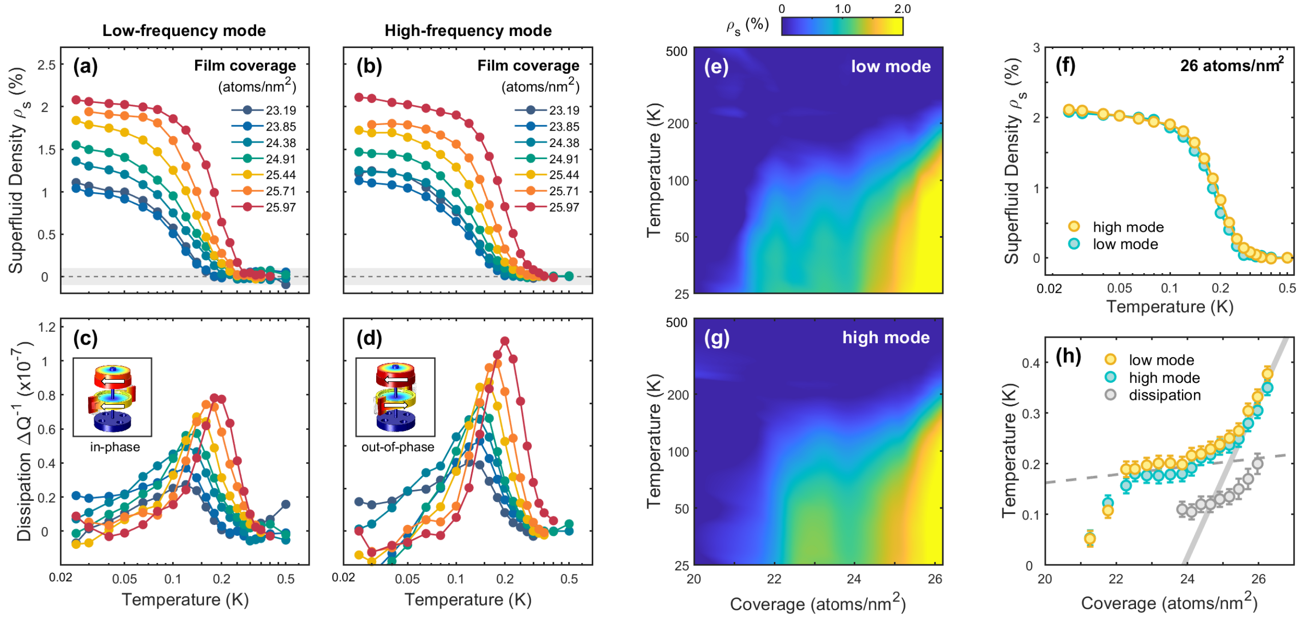


**Supplementary Fig.** 3. **Superfluidity in the third layer of $^4$He films.** Temperature dependence of superfluid density $\rho_s(T,n) = \delta P/\Delta P$ for (a) the low-frequency and (b) the high-frequency modes and dissipation $\Delta Q^{-1}$ for (c) the low-frequency and (d) the high-frequency modes, measured at different coverages. The sample color-coded curves are measured at the same coverage, respectively. The insets in (c) and (d) represent the displacement of the TO components calculated by a finite-element method simulation. $\rho_s(T,n)$ measured in the third layer shows a typical temperature-dependent characteristics expected in the BKT superfluid transition - a sudden jump or a rapid increase in $\rho_s(T)$ at the onset temperature due to vortext-antivortex unbinding, followed by shallow phonon contribution with $T^2$ dependence at low temperature. Temperature-dependent evolution of dissipation $\Delta Q^{-1}$ observed near the temperature where $\rho_s(T,n)$ changes most drastically at different coverage is also consistent with BKT phase transition. False-color two-dimensional mapping of $\rho_s$ as a function of temperature $T$ and the coverage $n$ in (e) the low-frequency and (g) the high-frequency modes. (f) Temperature dependence of the superfluid density $\rho_s$ at 26.0 atoms/nm$^2$ measured in both frequency modes are superimposed with each other. This plot confirms that the TO period reduction $\delta P/\Delta P$ for genuine superfluid transition is independent of frequency. (h) Superfluid onset temperatures $T_s(n)$ in the third layer. The grey solid line is the linear function $T_s(n) = 0.156(n - n_0)$ where $n_0 = 23.8$ atoms/nm$^2$ is the inert layer coverage for the third layer. This growth rate is consistent with that of the the BKT superfluid adsorbed on mylar substrate [21] and also that of the second layer of $^4$He films on graphite measured in this work.

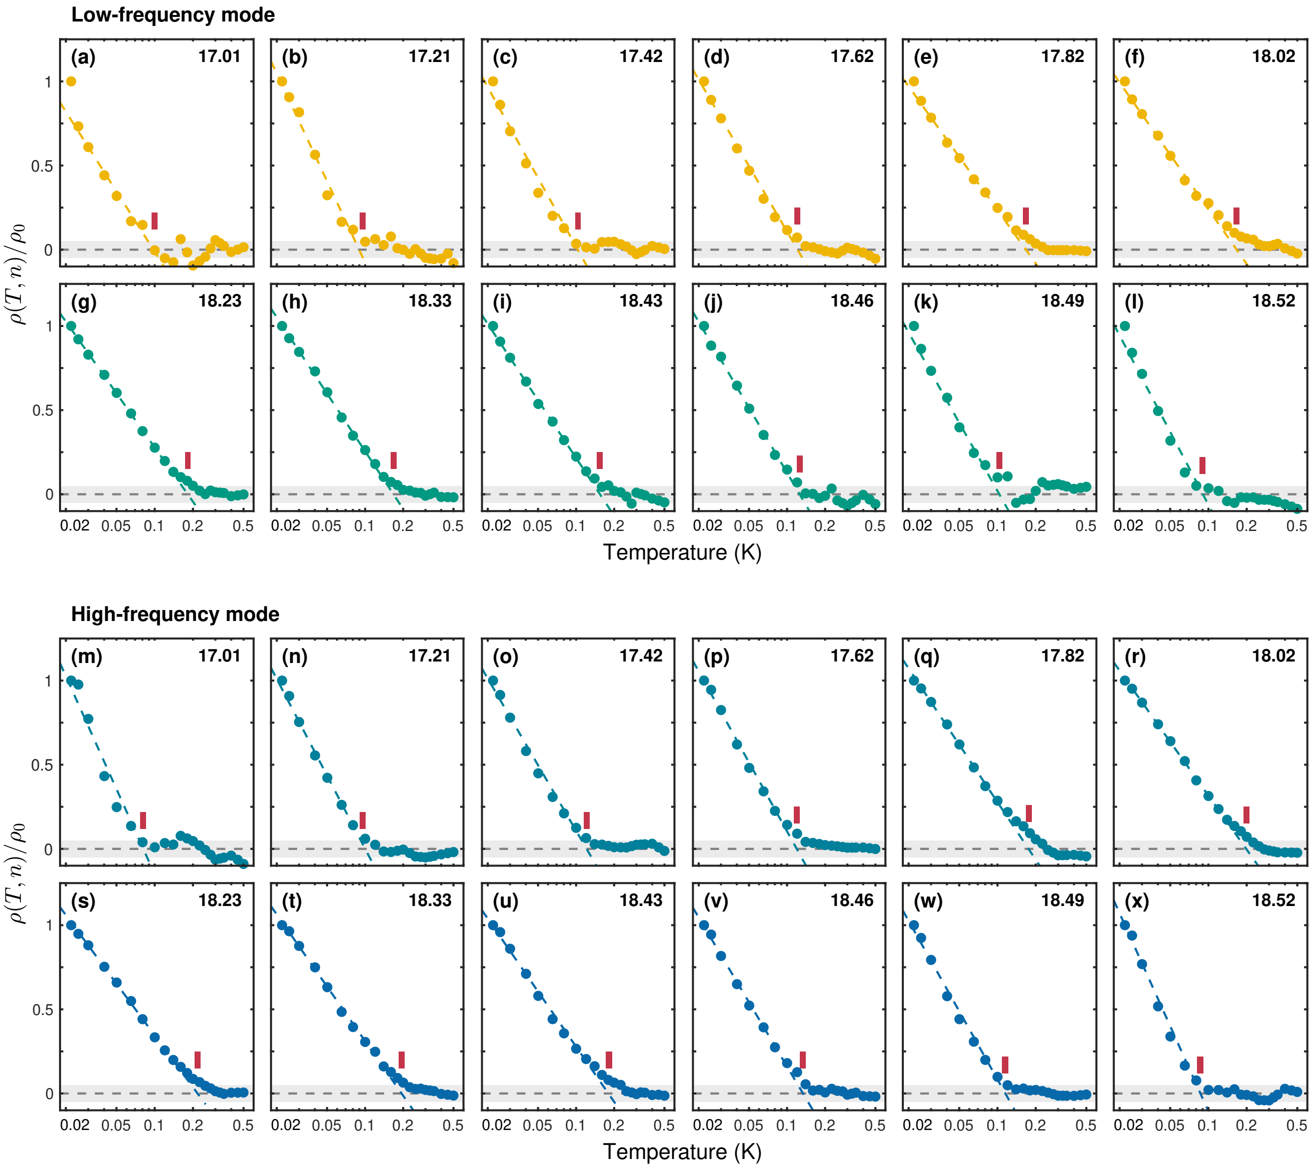


**Supplementary Fig.** 4. **Determination of superfluid onset temperature.** Superfluid onset temperature $T_s$ in the second layer is not determined straightforwardly due to its slow onset behavior (see main text). In order to systematically determine $T_s(n)$, the low-temperature trends of superfluid density $\rho_s$ are fitted with a linear function at each coverage in (a)-(l) the low-frequency and (m)-(x) the high-frequency modes. The fitted lines are presented by dashed lines in each panels. $T_s(n)$ in the second layer is then defined at temperatures where this fitted line meets $\rho_s = 0$ (thick red bars).
